# Supplementary material for: ImageInThat: Manipulating Images to Convey User Instructions to Robots
Source: arXiv:2503.15500 source file (2025-01-21)
Supplement: Supplementary file 2 [file 9-appendix.tex]

\section*{Appendices}

\subsection{Prompts}
Here we list the LLM prompts used for various functionalities of \projname. 
We focus on the main system components, including environment representation, program generation, and user goal prediction.

%\noindent \emph{Environment Representation}
\subsubsection{Environment Representation} ~\label{sec:appendix-env-rep}
The environment representation in \projname includes a list of objects and fixtures and their states.
The objects and fixtures are stored as a dictionary, where each object or fixture is indexed by its name. 

\noindent \emph{Objects} Objects are tracked in the following json format:

\{``class'': \texttt{String},
``boundingBox'': \texttt{[Number]},
``category'': \texttt{String},
``isReceptacle'': \texttt{Boolean},
``width'': \texttt{Number},
``height'': \texttt{Number},
``image'': \texttt{Byte (base64)}\}

\noindent \emph{Fixtures}
Fixtures are represented as:

\{``class'': \texttt{String},
``boundingBox'': \texttt{[Number]},
``category'': \texttt{String},
``width'': \texttt{Number},
``height'': \texttt{Number},
``x'': \texttt{Number},
``y'': \texttt{Number},
``possibleStates'': \texttt{[String]}\}

\noindent \emph{Environment States}
Finally, the state dictionary tracks the transient states of the environment and user input, in the format of 
\{``caption'': \texttt{String},
``objects'': \texttt{Object state dictionary},
``fixtures'': \texttt{Fixture state dictionary},
``objectOrder'': \texttt{[String]}
\}

The object state dictionary stores the x, y coordinates of individual objects, as {\{``x'': \texttt{Number}, ``y'': \texttt{Number}\}}.
The fixture state dictionary stores the current state of each fixture, as {\{``state'': \texttt{String}\}}.
Both dictionaries have object or fixture names as their keys.

\subsubsection{Captioning}
We caption the state change induced by users' manipulation of environment images with the following prompt:

\vspace{4pt}
\noindent\hrule
\vspace{2pt}

[Rules]:
You are a helpful assistant to a robot trying to figure out what language instruction it needs to perform.
You are provided the current environment state that describes all the objects and fixtures in the scene.
You are also given a current image and envState whch describes the location of all objects as well as the state of fixtures.
Given the current and next image (plus data), provide [Reasoning] about what was changed between them.
In the case when an object moves, be specific about which objects move and where they move to.
For instance, if there are two identical objects one on the left and another on the right, state which object (e.g., left most object) moved.
if there are objects inside other objects (e.g., food on a plate), mention both the food and the plate.
Once you finish [Reasoning], state the [Instruction] that would be required to execute the change between the images.
Respond with the term [Instruction] and provide a one-line description.
You should use descriptive language like `on the left of' or 'inside of' or 'the red colored object'.
However, do not explicitly include coordinates in your response.
Here's an example response.
[Instruction]:
``Put the apple on the left side of the cabinet into the bowl on the right.''

\vspace{2pt}
\noindent\hrule
\vspace{4pt}

This prompt is appended with environment information, and the environment states of the current and next step (i.e. after user manipulation), as described by Appendix~\ref{sec:appendix-env-rep}. 
Specifically, they follow the format of: 

%\vspace{4pt}
%\noindent\hrule
%\vspace{2pt}
[Environment]: \texttt{environment object}

[Current Environment State]: \texttt{Current environment state object}

[Next Environment State]: \texttt{Next environment state object}
%\vspace{2pt}
%\noindent\hrule
%\vspace{4pt}

% \subsection{Program Creation}
% We use the following prompt to the LLM for creating a program, based on the user's manipulation of the environment images and the current environment states.

% \vspace{4pt}
% \noindent\hrule
% \vspace{2pt}

% [Rules]:
% You are a helpful assistant to a robot arm trying to perform manipulation tasks.
% Below, you are provided information about a sequence of instructions that a human provided.
% Each step in the sequence consists of an image and a data representation of all the objects and fixtures in the environment and their locations.
% Objects are items that can be moved around (e.g., a fruit) while fixtures are items that change state (e.g., a drawer that can open or close).
% Given this sequence, try to describe what is happening in each step under [Reasoning].
% Then, generate a [Response] that describes the higher-level logic that the instructions are attempting to communicate.
% The goal is to generate logic that can be used even if the environment has changed or there are different objects and fixtures.
% The response should be a few lines at most describing what the robot should do to achieve the goals seen in the instructions.
% \vspace{2pt}
% \noindent\hrule
% \vspace{4pt}

% The prompt above will be appended with the user manipulation and environment image at every step involved.
% The user manipulation description at Step \textit{i} follows the format of:

% ``[Step (\textit{i})]: \texttt{String}''

\subsection{User Goal Prediction}

We use the following prompt to predict the user's goal and suggest possible robot actions as a form of auto-completion:

\vspace{4pt}
\noindent\hrule
\vspace{2pt}

Rules:
You are a helpful assistant to a fixed robot arm that is trying to complete a task. 
The robot arm in this environment has the following skills:
1. Place/put an item somewhere.
2. Open/close drawers.
3. Open/close cabinets.
4. Open/close microwave doors.
5. Turn a stove on/off.
6. Press a button on a coffee machine.
7. Turn on/off sink faucet.
8. Turning the sink spout.
The robot cannot lift heavy items.
You are provided with data that correponds to what the robot's environment looks like, plus a bunch of step that the robot wants to get to.
Each step consists of an image observation from the robot's sensors.
Each step also consists of a structured representation of the environment state at that moment, including the location of all objects and the fixture's states.
Start by providing a [Summary] stating what happened in each step.
Given this information for each step in sequence as well as information about objects and fixtures, predict what the robot is attempting to do.
Then, predict one or two independent logical steps that make sense in the context of the environment and sequence of steps. Predict two steps if there are many options. Predict one step if there is only one good option.
These predicted steps should not be sequential. 
For each predicted step, state why that step would actually happen.
Then, determine if the instruction requires a change in the background or manipulating objects.
Changing the background is required when the state of fixtures needs to change (e.g., turning on/off a light).
if changing a background is required, do not output anything.
Manipulating objects is required when the instruction implies that object(s) need to move somewhere.
Respond in natural language.
Before responding, provide your [Reasoning] and concretely state what objects or fixtures might be manipulated next.
Then, provide your [Response] with each entry in a new line and enumerated.
Only use items that are present in the environment in these imagse to predict those steps. 
Do not introduce new items that are not visible in the images.
Each step should involve a single item (e.g., a banana).
Do not provide multiple options within a single step (e.g., x or y).
Output the response as a list of dictionaries.
Do not return the word `json' when returning the output.
In each dictionary, include `action' and `change\_needed' as a key.
`action' indicates the instruction for the robot.
`change\_needed' can either be `Change background' or `Move objects'. Do not output anything else.
Describe the action in natural language (do not use numbers to refer to objects). But be descriptive about what needs to happen.
The robot cannot stop the task.

\vspace{2pt}
\noindent\hrule
\vspace{4pt}

\subsection{Experimental Tasks and Oracles}

The following are the prompts given to participants as they completed the study for each task, and the oracles for each task used to measure errors.

\subsubsection{Storing Pantry}

You just got home from buying some groceries. You want the robot to stock your pantry so that all items are easily accessible.

\begin{figure}[h!]
    \centering
    \includegraphics[width=0.95\linewidth]{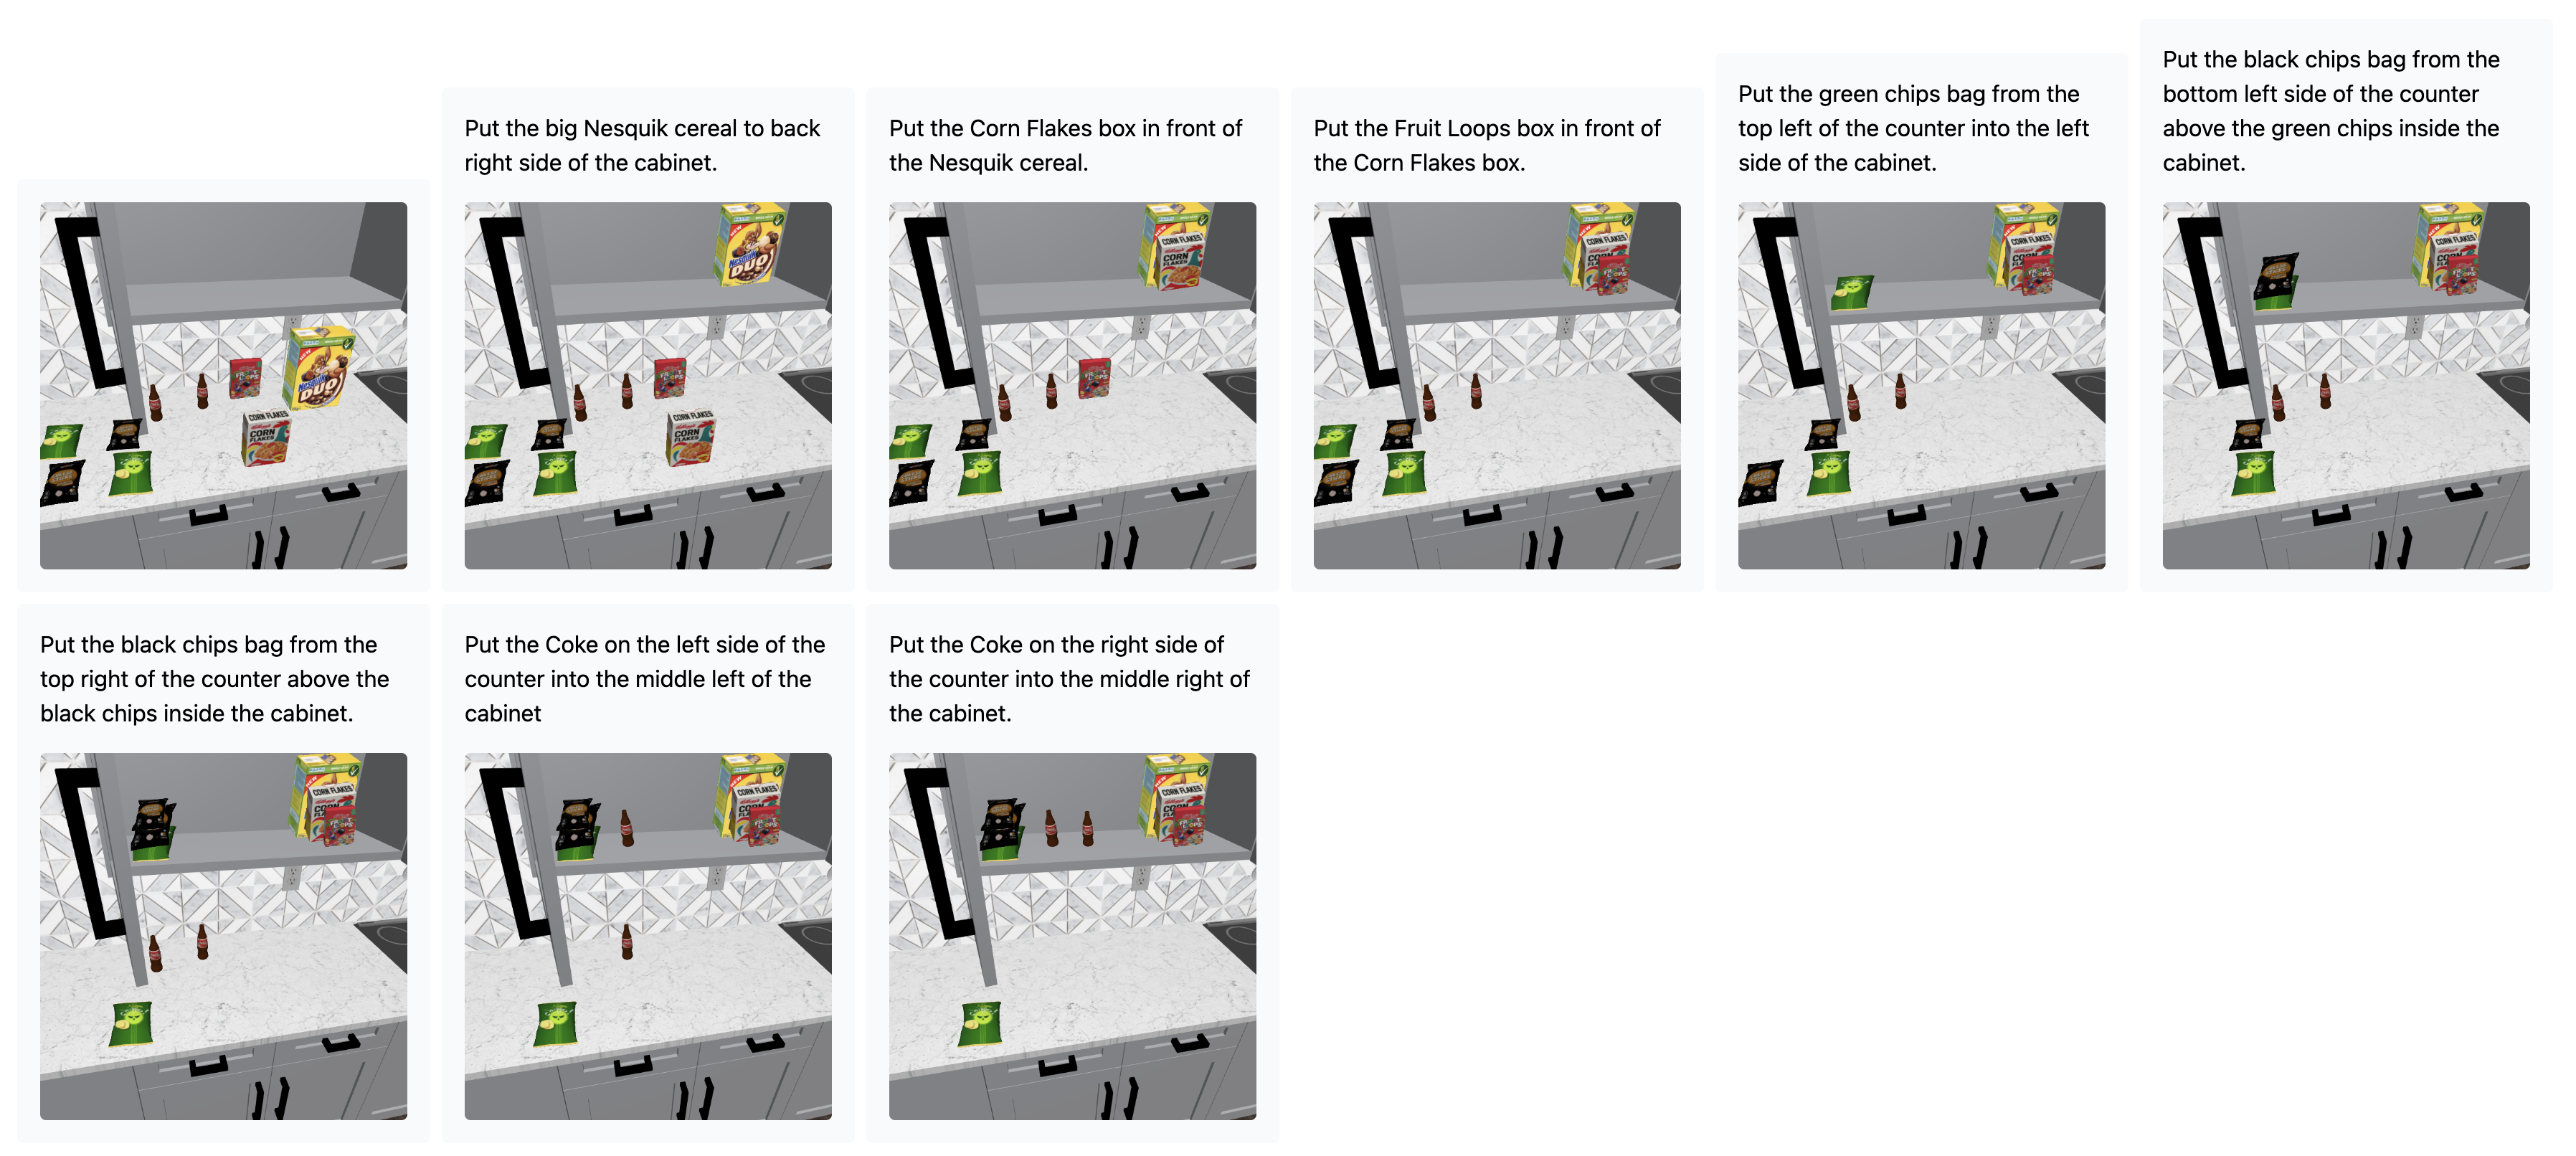}
    % \caption{System diagram of \projname showing the 1. server, 2. client, and 3. robot.}
    \label{fig:storing-oracle}
\end{figure}

\begin{itemize}
\item Item categories: [cereal, chips, soda, cabinet]
\item Organize the cereals by height so they are all visible.
\item Chips take up a lot of space but are soft. Stack them by flavor, but keep one packet of the green chips on the counter to eat now.
\item Organize your soda bottles so that the label is always visible.
\item Do not let items of different categories touch each other.
\item Do not perform any actions that are not explicitly mentioned in the requirements.
\end{itemize}

\subsubsection{Sorting Fruits}

You are trying to organize your unripe and ripe fruits. This includes unripe bananas and ripe bananas. This also includes unripe apples (green tint) and ripe apples (red). You want to make applesauce with the ripe apples.

\begin{figure}[h!]
    \centering
    \includegraphics[width=0.95\linewidth]{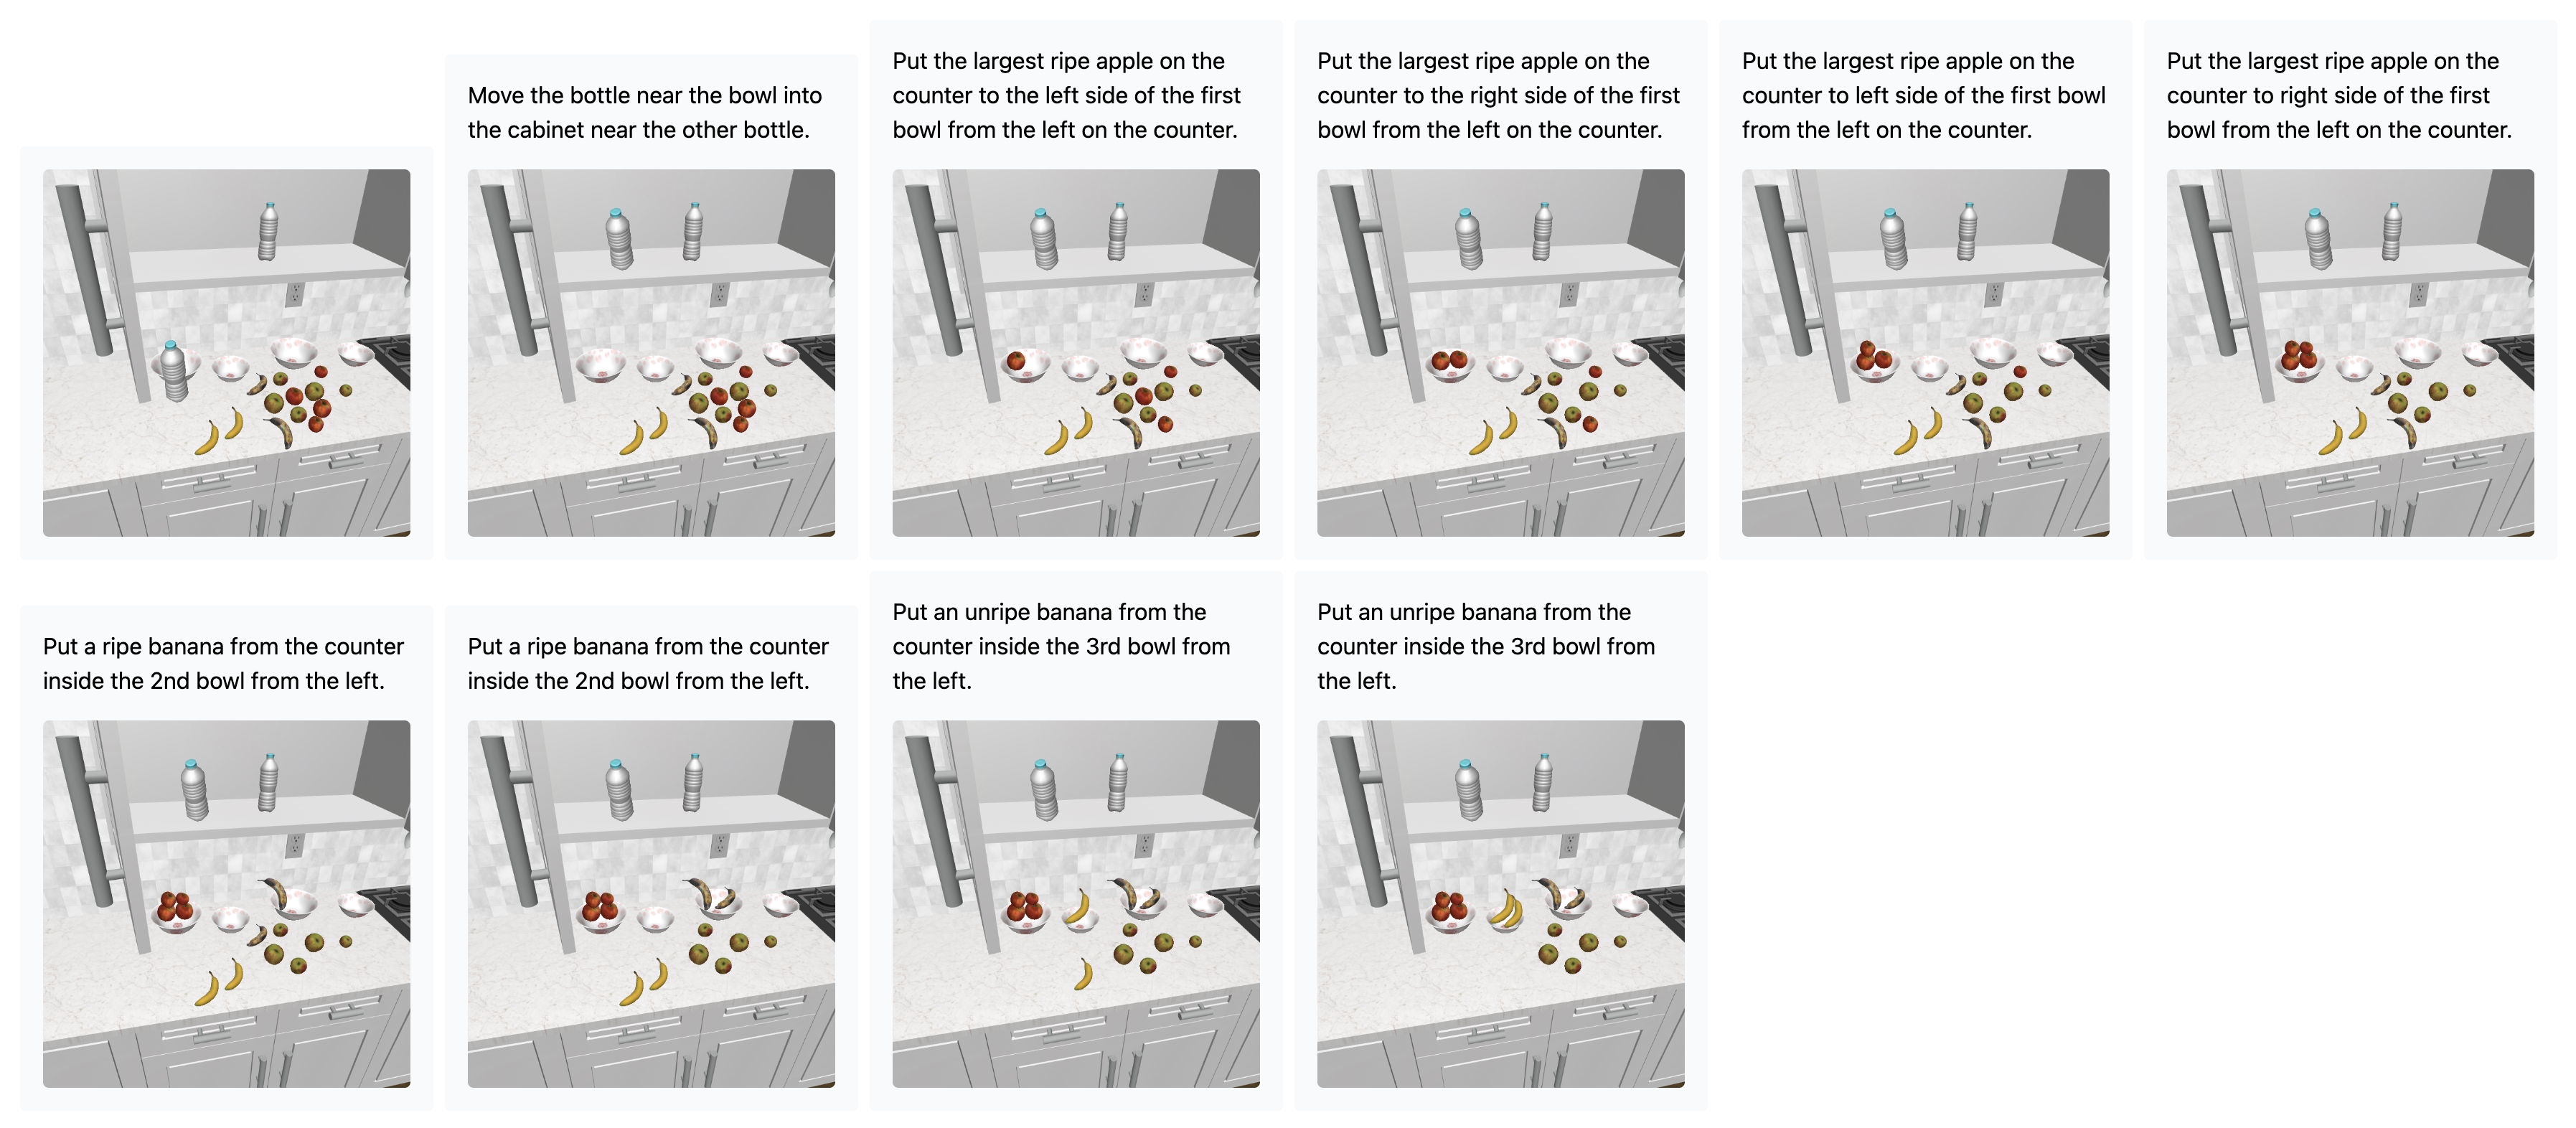}
    % \caption{System diagram of \projname showing the 1. server, 2. client, and 3. robot.}
    \label{fig:sorting-oracle}
\end{figure}

\begin{itemize}
\item Item categories: [unripe bananas, ripe bananas, unripe apples (green tint), ripe apples (red)]
\item A bottle is blocking the bowls so put it away in the right location.
\item Arrange the ripe apples in one bowl ensuring the smaller ripe apples are not crushed by the larger ripe ones.
\item Sort the unripe and ripe bananas into separate bowls.
\item Leave the unripe apples on the counter as they are not needed for the applesauce.
\item Do not perform any actions that are not explicitly mentioned in the requirements.

\end{itemize}

\subsubsection{Cooking Stir-fry}

You are trying to make a quick, but mild veggie stir fry to eat with dinner. You want to use olive oil in cooking because it is healthy.

\begin{figure}[h!]
    \centering
    \includegraphics[width=0.95\linewidth]{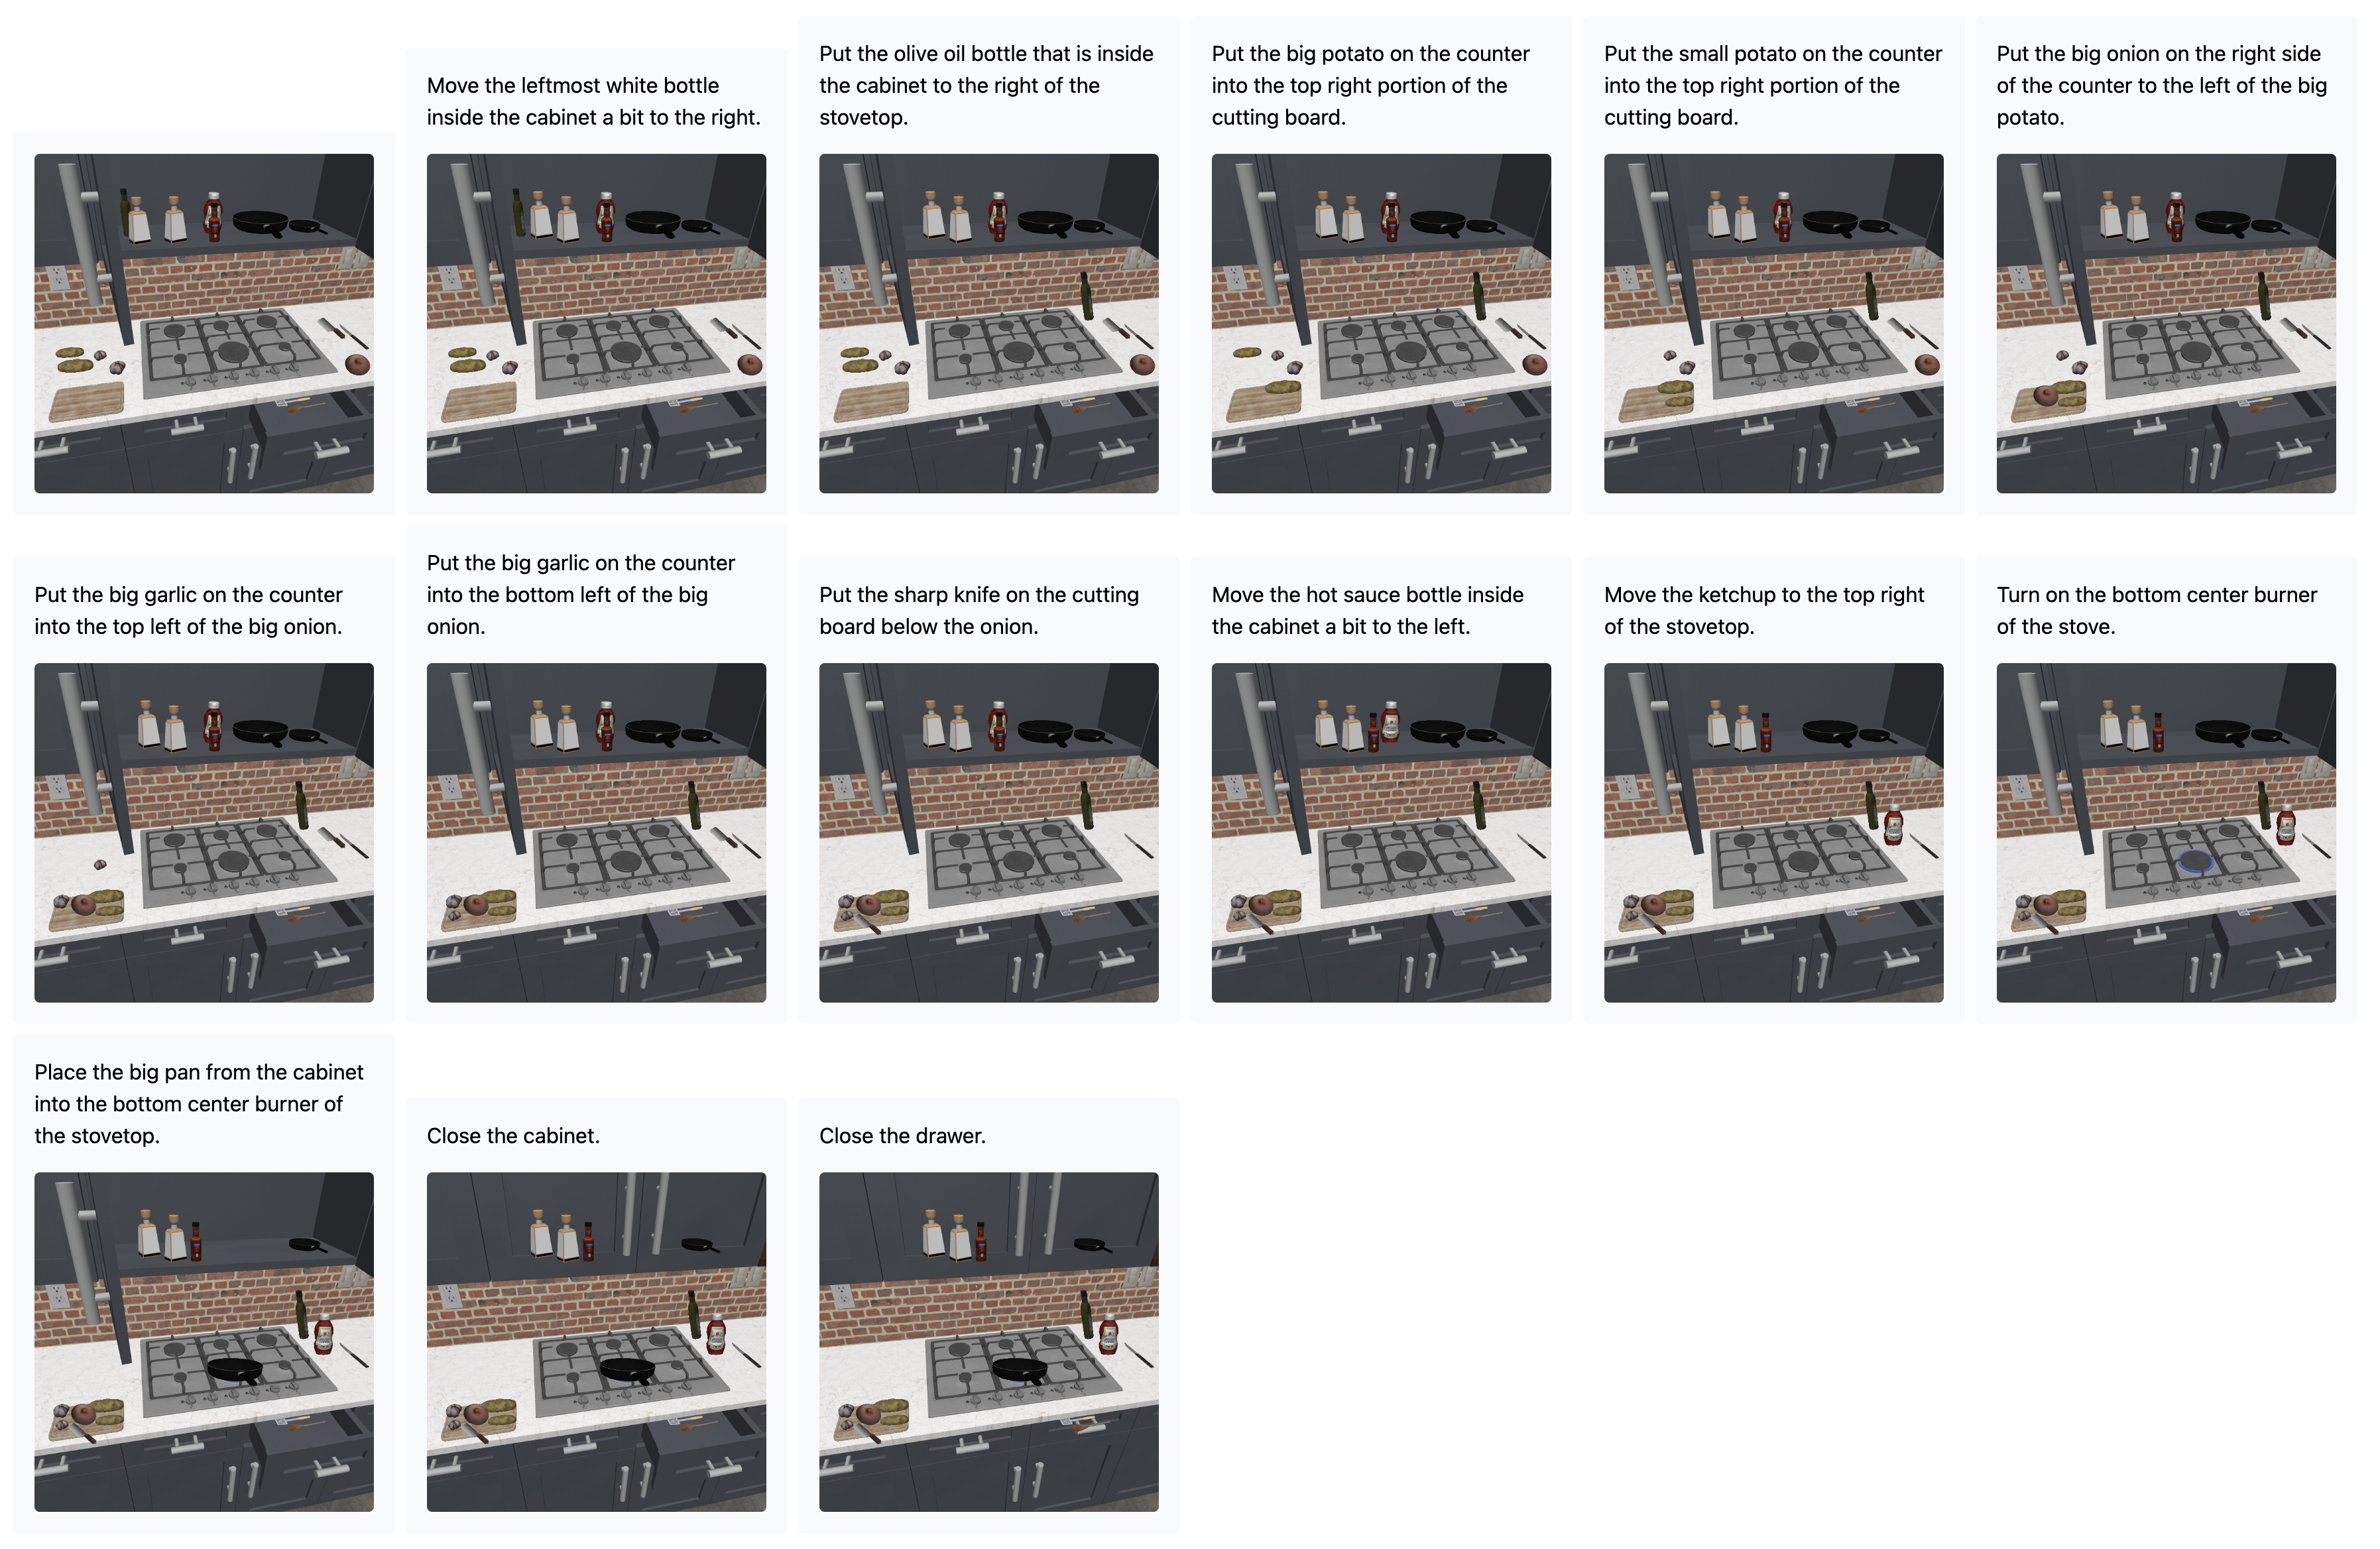}
    % \caption{System diagram of \projname showing the 1. server, 2. client, and 3. robot.}
    \label{fig:cooking-oracle}
\end{figure}

\begin{itemize}
\item Item categories: [vegetables, olive oil (green), other bottles, hot sauce, ketchup, knifes, stove, pan, spatula, cabinet]
\item The olive oil (green bottle) is blocked by the other oil bottles. Make space and put it close to where you will be cooking.
\item Organize your vegetables on the cutting board so that they are placed in the order in which they will be put in the pan: 1. Potatoes, 2. Onions, 3. Garlic.
\item For vegetables of the same type, organize them on the cutting board by descending order in size.
\item You want to use a sharp knife to cut all the vegetables. Place it on the cutting board but without blocking the vegetables.
\item You prefer ketchup over hot sauce. Place it close to where you will be cooking.
\item You want to use a big pan to cook a lot of food. Turn on the burner that will cook the food most evenly using the big pan.
\item Put the big pan on the appropriate burner.
\item When you’re done, close everything.
\item Do not perform any actions that are not explicitly mentioned in the requirements.
\end{itemize}

\subsubsection{Washing Dishes}

You just threw a small party and the guests just left. You want the robot clean up the dishes while you get ready for bed.

\begin{figure}[h!]
    \centering
    \includegraphics[width=0.95\linewidth]{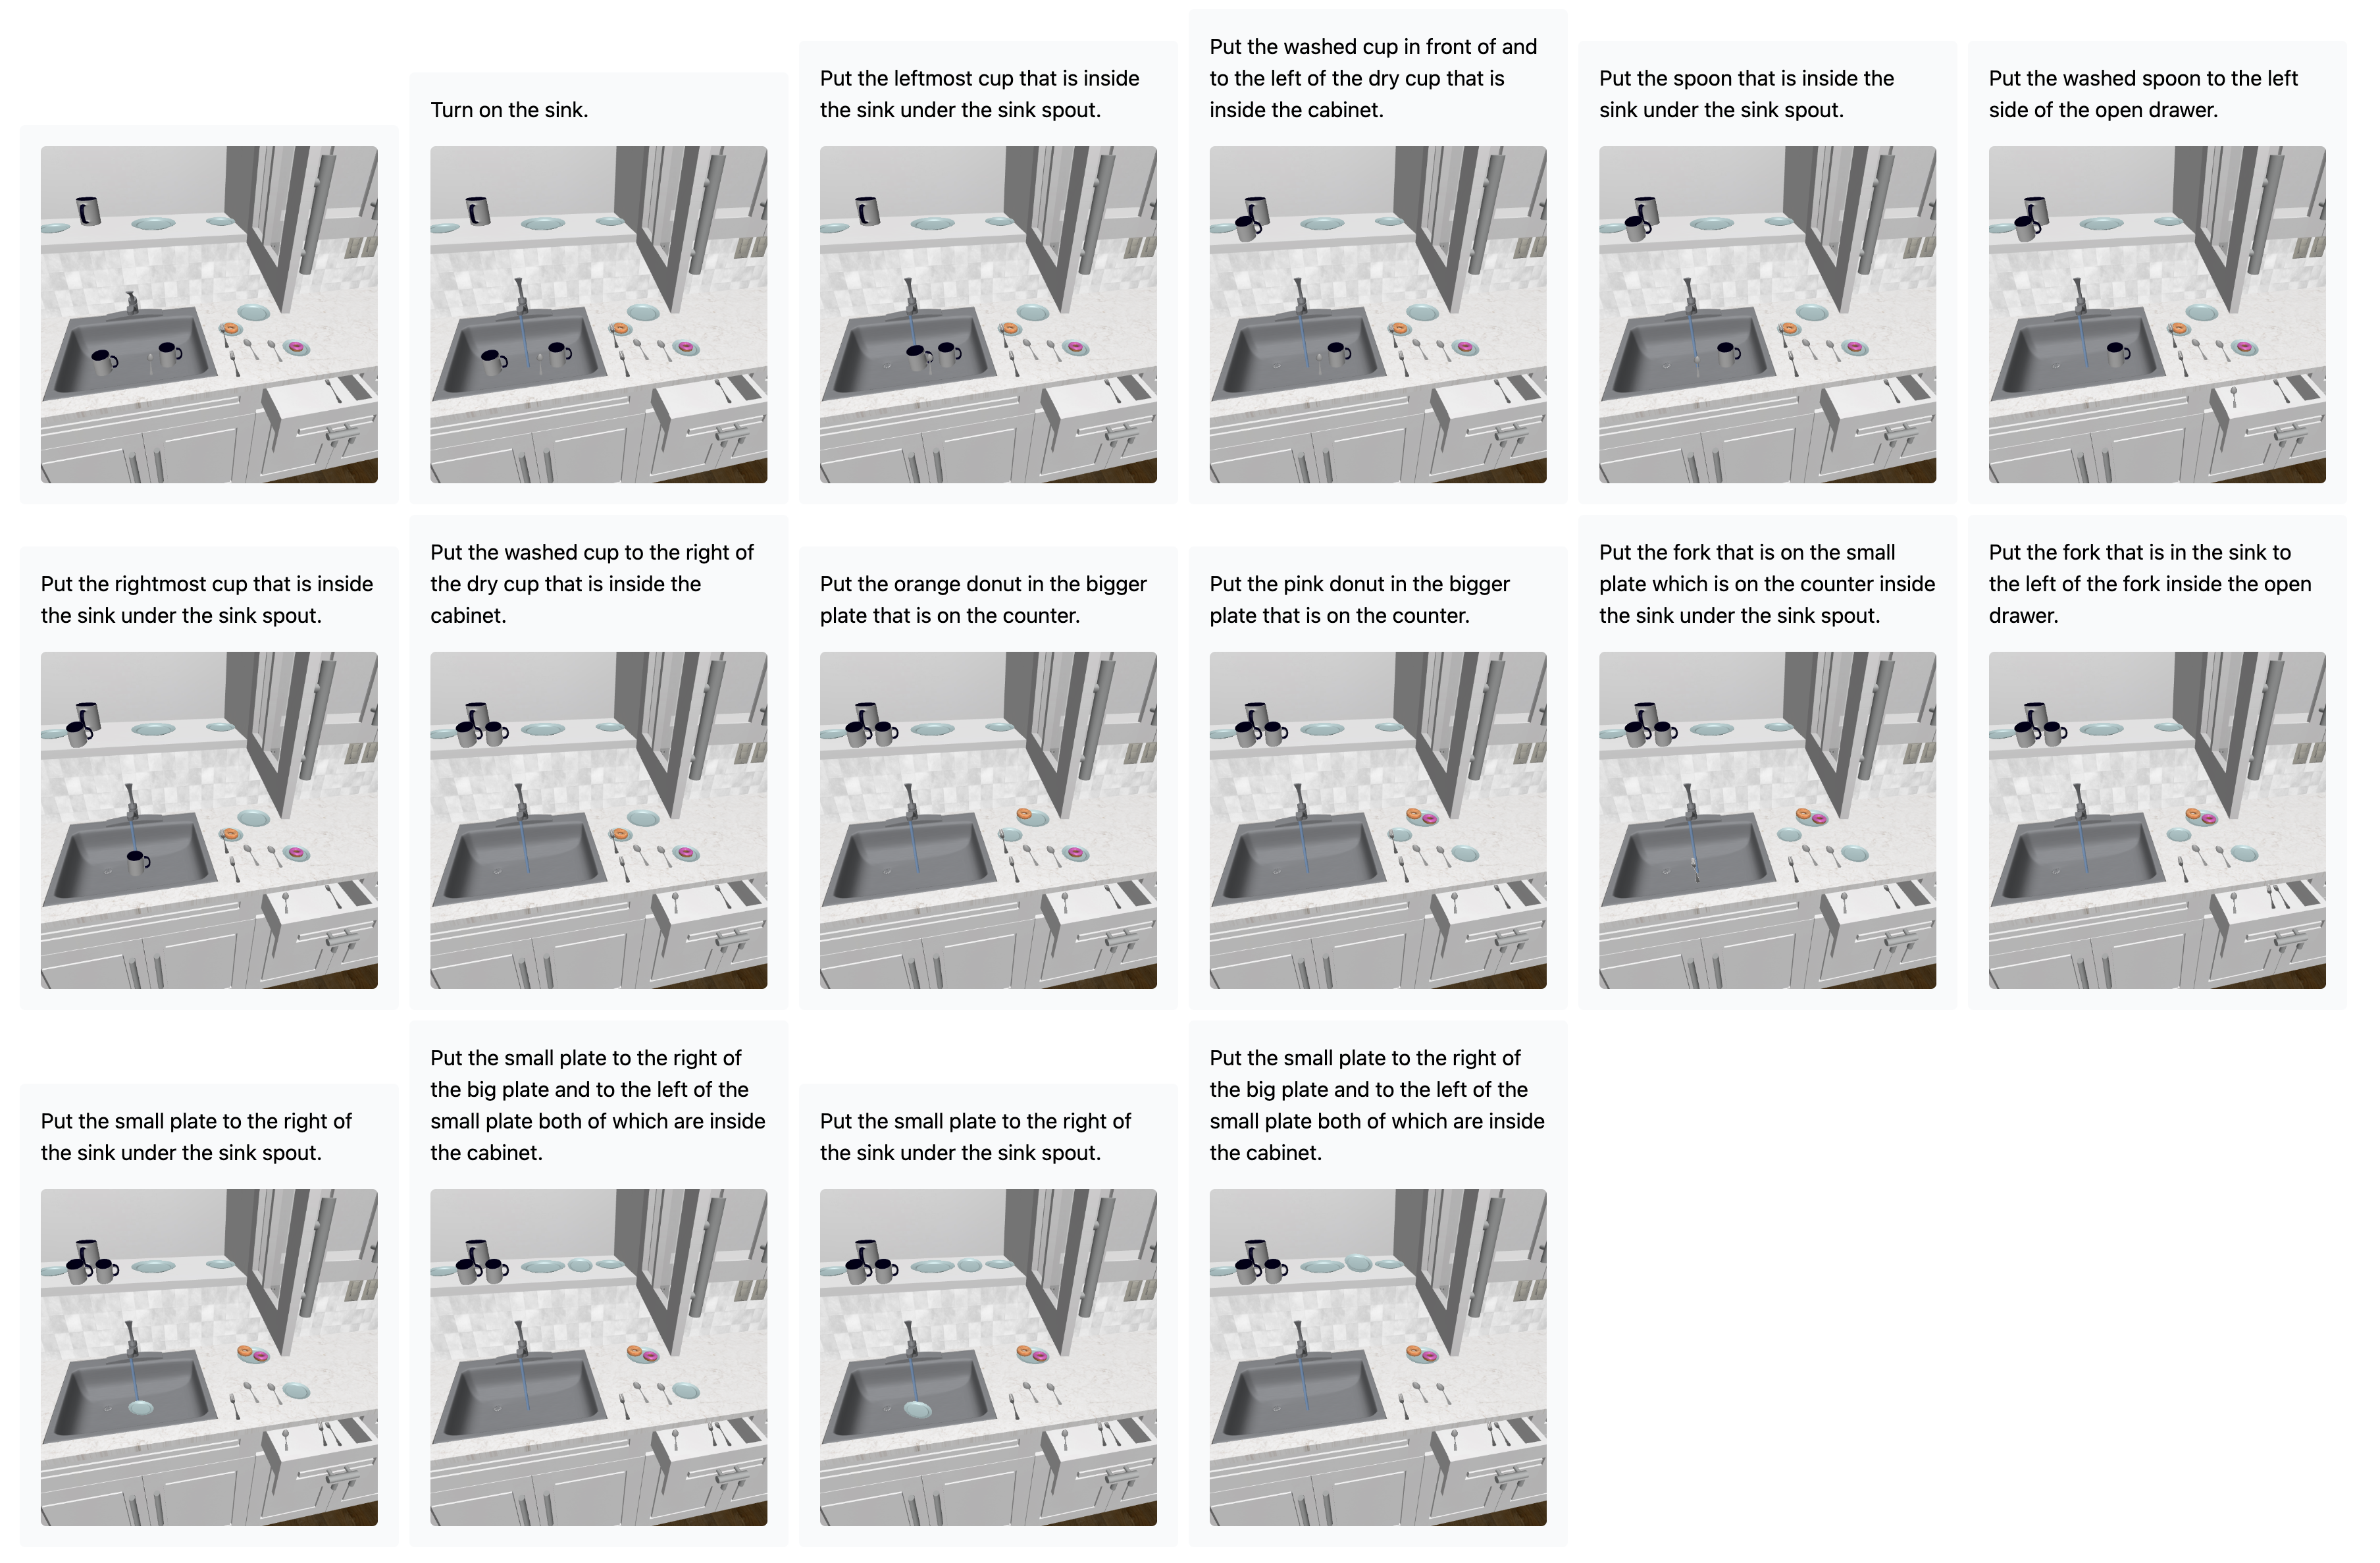}
    % \caption{System diagram of \projname showing the 1. server, 2. client, and 3. robot.}
    \label{fig:dishes-oracle}
\end{figure}

\begin{itemize}
\item Item categories: [cups, small plates, big plates, spoons, forks, drawer, cabinet]
\item To rinse dishes, they must be placed directly underneath where the water flows.
\item After rinsing a cup or plate, they should be placed inside the cabinet but without making contact with dry dishes.
\item Rinsed utensils like forks and spoons should be put inside the drawer by grouping similar utensils (e.g., fork-fork-spoon-spoon).
\item Cups and spoon that are already in the sink should be rinsed and placed in the appropriate areas.
\item Transfer the donuts to the bigger plate so that you can clean the smaller plates.
\item Clean all plates and forks that made contact with the donuts.
\item Do not perform any actions that are not explicitly mentioned in the requirements.
\end{itemize}

%\vspace{20pt}

\subsection{Oracle Comparison Interface}
To determine the various types of errors made by participants, we created an interface (\autoref{fig:judging-interface}) for loading the participants' data to compare it to the ground truths. The interface allowed us to quickly drag and drop tasks to sort them and had features to quickly assign the next unfilled subtask by double-clicking on a step.

\begin{figure}[h!]
    \centering
    \includegraphics[width=0.95\linewidth]{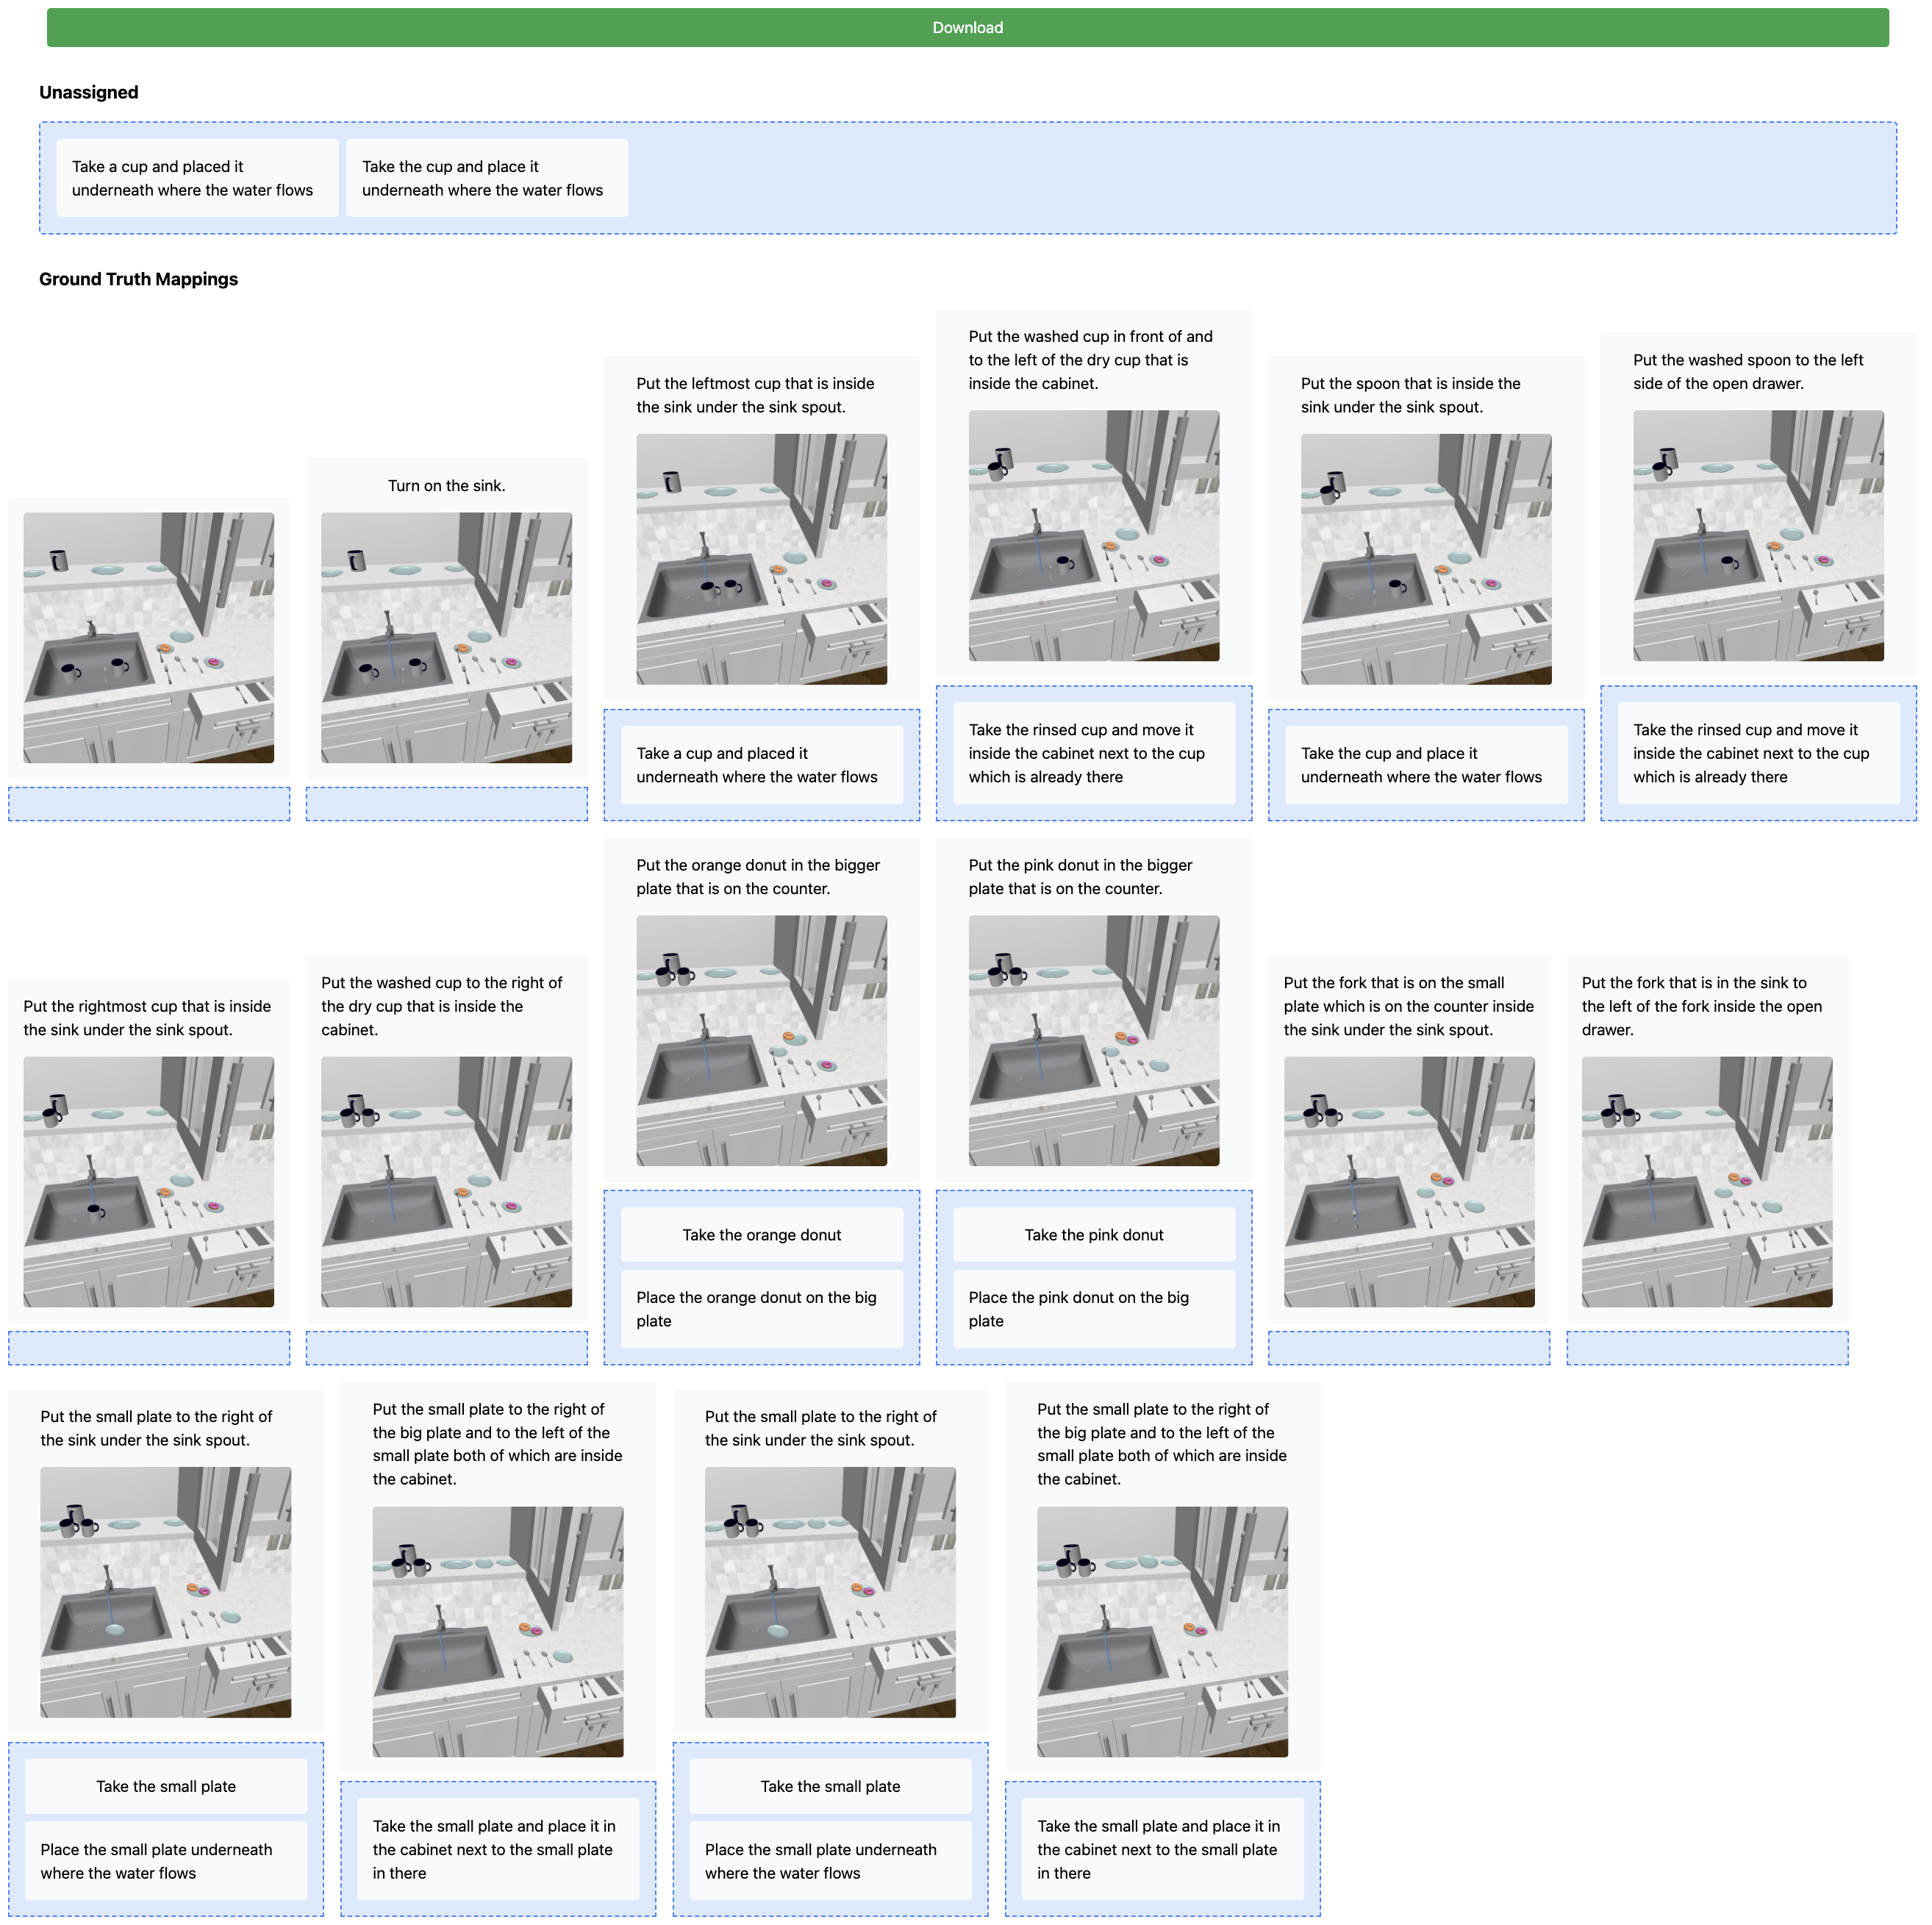}
    \caption{The interface used to judge participant data. The displayed data demonstrates a participant who made all three types of errors. The textual instructions in the unassigned section are extraneous, any empty blue box are missing instructions, and blue boxes with multiple instructions are inefficient. The text and image above each blue box are our oracle data.}
    \label{fig:judging-interface}
\end{figure}
